# Supplementary material for: Abductive Ego-View Accident Video Understanding for Safe Driving Perception
Source: arXiv:2403.00436 source file (2024-03-01)
Supplement: Supplementary file 1 [file suppl.tex]

\clearpage
\setcounter{equation}{0}
\setcounter{figure}{0}
\setcounter{table}{0}
\setcounter{page}{1}
\setcounter{section}{0}

\twocolumn[{%
\renewcommand\twocolumn[1][]{#1}%
\maketitle
\begin{center}
    \textbf{\Large Supplementary Material of Residual Pattern Learning for Pixel-wise Out-of-Distribution Detection in Semantic Segmentation}
    \vspace{20pt}
\end{center}
\maketitle

\section{Rationale}
\label{sec:rationale}

    \begin{figure*}[!t]
  \centering
\includegraphics[width=0.9\linewidth]{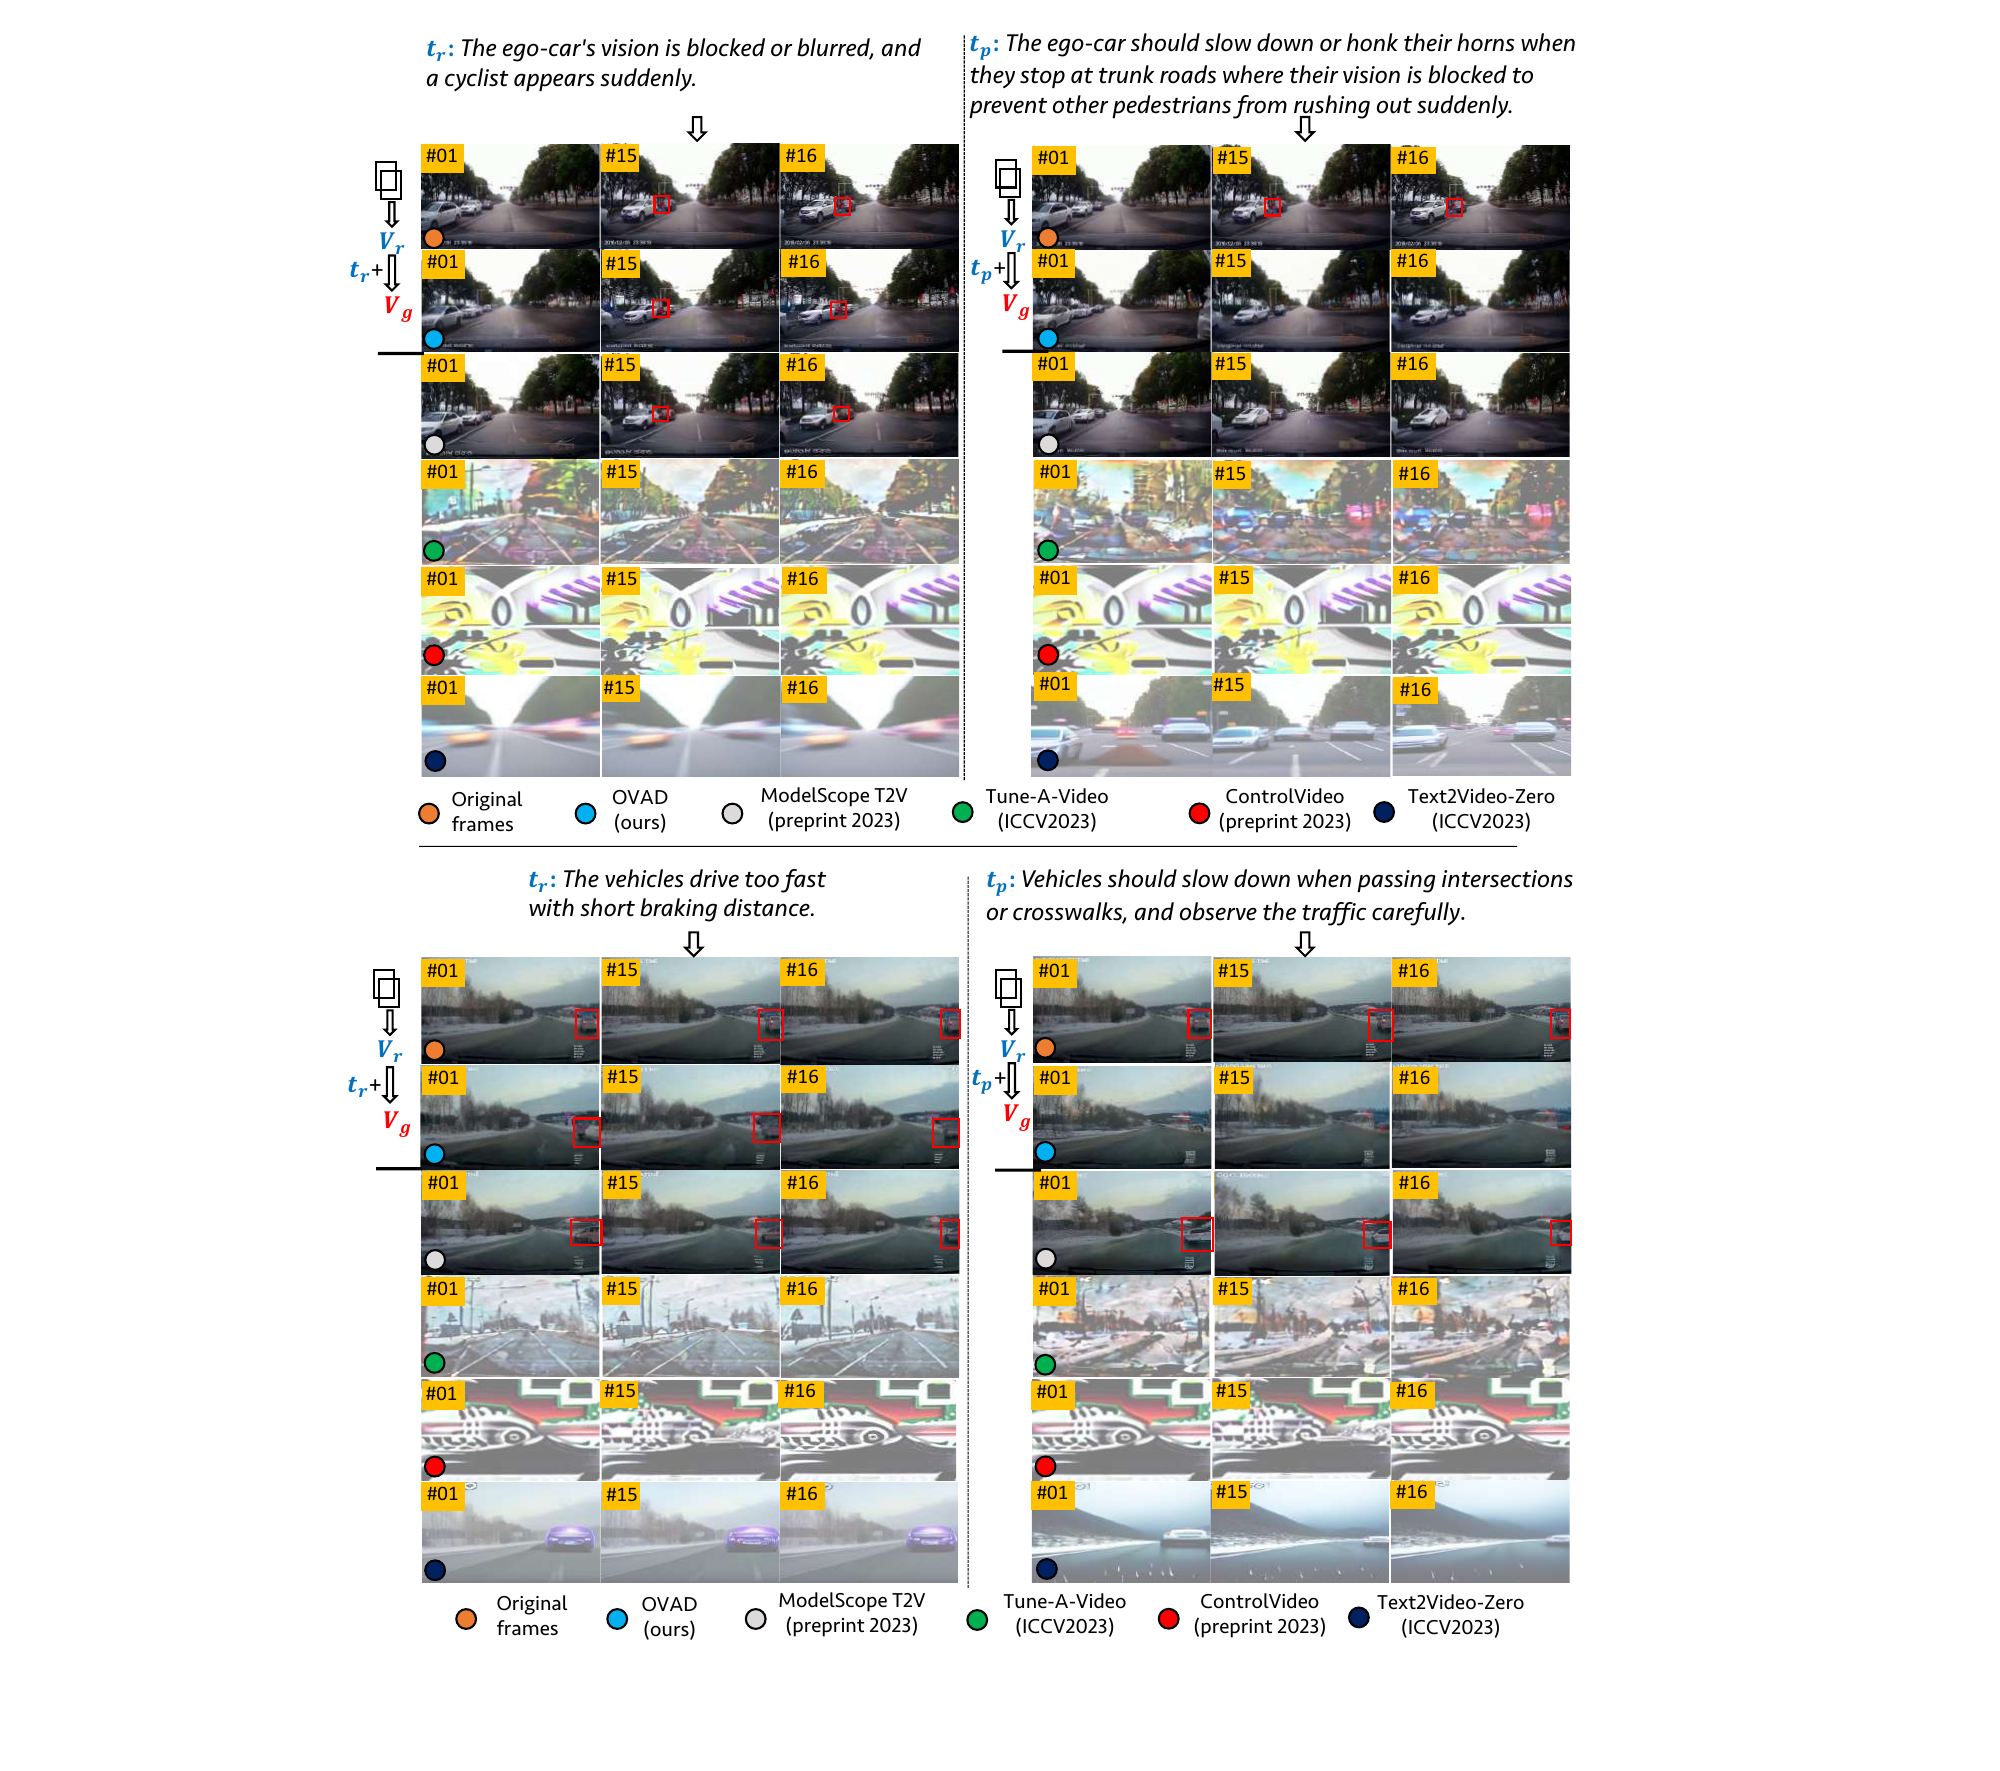}
   \caption{\small{The visualization of video diffusion by our OAVD, ModelScope T2V \cite{ModelScopeT2V}, Tune-A-Video \cite{wu2023tune}, ControlVideo \cite{zhang2023controlvideo}, and Text2Video-Zero \cite{text2video-zero}.}}
   \label{fig13}
   \vspace{-0.5em}
\end{figure*}
Having the supplementary compiled together with the main paper means that:
\begin{itemize}
\item The supplementary can back-reference sections of the main paper, for example, we can refer to \cref{sec:intro};
\item The main paper can forward reference sub-sections within the supplementary explicitly (e.g. referring to a particular experiment); 
\item When submitted to arXiv, the supplementary will already included at the end of the paper.
\end{itemize}
To split the supplementary pages from the main paper, you can use \href{https://support.apple.com/en-ca/guide/preview/prvw11793/mac#:~:text=Delete%20a%20page%20from%20a,or%20choose%20Edit%20%3E%20Delete).}{Preview (on macOS)}, \href{https://www.adobe.com/acrobat/how-to/delete-pages-from-pdf.html#:~:text=Choose%20%E2%80%9CTools%E2%80%9D%20%3E%20%E2%80%9COrganize,or%20pages%20from%20the%20file.}{Adobe Acrobat} (on all OSs), as well as \href{https://superuser.com/questions/517986/is-it-possible-to-delete-some-pages-of-a-pdf-document}{command line tools}.
